# Supplementary material for: On the Boroxol Ring Fraction in Melt-Quenched B$_2$O$_3$ Glass
Source: arXiv:2512.14526 ancillary file (2025-12-16)
Supplement: Supplementary file 1 [file si.pdf]

# Supporting Information: On the Boroxol Ring Fraction in Melt-Quenched $B_2O_3$ Glass

Debendra Meher, Nikhil V. S. Avula, and Sundaram Balasubramanian*

*Chemistry and Physics of Materials Unit, Jawaharlal Nehru Centre for Advanced Scientific Research, India*

E-mail: bala@jncasr.ac.in

# Contents

**S1 Relevant Experimental Data from Literature** **3**

S1.1 Experimental Data: Mass Density Versus Temperature . . . . . . . . . . . . 3

S1.2 Experimental Data: Boroxol Fraction & Viscosity Versus Density . . . . . . 4

**S2 Summary of Simulations Literature on Boroxol Yield in $B_2O_3$ Glasses** **4**

**S3 MLP Refinement** **6**

S3.1 High Boroxol Dataset Collection . . . . . . . . . . . . . . . . . . . . . . 6

S3.2 DeePMD MLP training . . . . . . . . . . . . . . . . . . . . . . . . . . . 8

S3.3 DeePMD Hyperparameter testing . . . . . . . . . . . . . . . . . . . . . . 9

S3.4 MACE training . . . . . . . . . . . . . . . . . . . . . . . . . . . . . . . 10

S3.5 MACE Hyperparameter testing . . . . . . . . . . . . . . . . . . . . . . . 10

**S4 MLP validation: Equation of State of Crystals** **11**

S4.1 Pressure versus MLP descriptor range cut-off . . . . . . . . . . . . . . . . 14

**S5 Structural Analysis** **15**

**S6 Results** **20**

S6.1 Quenching at Constant Volume: NVT . . . . . . . . . . . . . . . . . . . . 20

S6.2 Results: Variable Quench Rates . . . . . . . . . . . . . . . . . . . . . . . 22

S6.3 Vibrational Spectra . . . . . . . . . . . . . . . . . . . . . . . . . . . . . 25

S6.4 Generation of amorphous configurations over a wide range of boroxol fractions 26

S6.5 Boroxol Formation Visualization . . . . . . . . . . . . . . . . . . . . . . 26

S6.6 Boroxol Melting . . . . . . . . . . . . . . . . . . . . . . . . . . . . . . . 28

S6.7 Negative Pressure . . . . . . . . . . . . . . . . . . . . . . . . . . . . . . 30

**References** **32**

# S1 Relevant Experimental Data from Literature

## S1.1 Experimental Data: Mass Density Versus Temperature

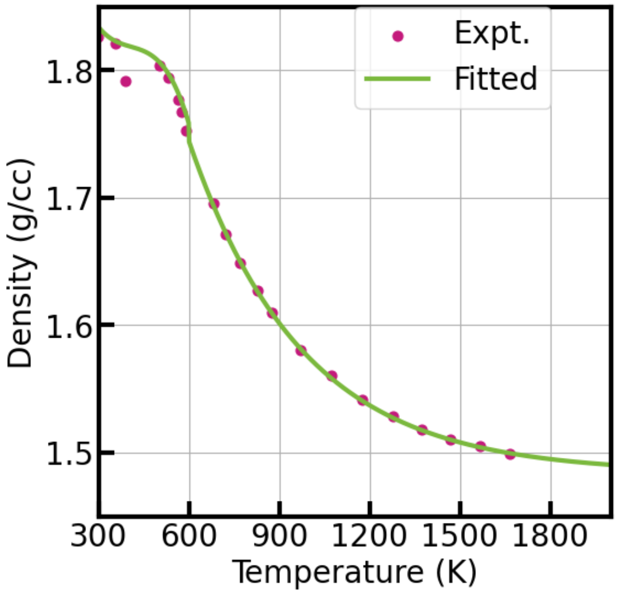


Figure S1: The experimentally measured temperature versus density data for $B_2O_3$ ranges from 2000 K to 300 K. The data (circles) were collected from two different sources: high-temperature data above 600 K were taken from Napolitano et al.,[1] while data below 600 K were sourced from Macedo et al.[2] The solid line is the fit to the data using two different equations.

The fit function to the temperature-dependent density is:

$$\rho(T) = \begin{cases} 1.28\, e^{-T/377} + 1.484, & \text{if } T > 600K \\ aT^3 + bT^2 + cT + 2.292, & \text{if } T < 600K \end{cases}$$

where

$$a = -6.59 \times 10^{-9},$$

$$b = 8.055 \times 10^{-6},$$

$$c = -3.35 \times 10^{-3}.$$

### S1.2 Experimental Data: Boroxol Fraction & Viscosity Versus Density

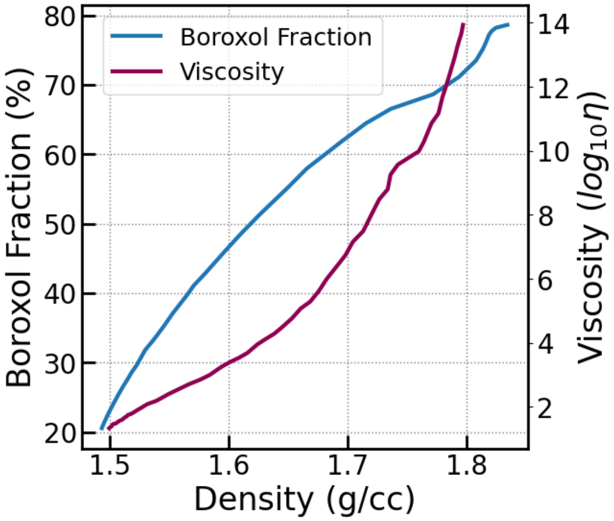


Figure S2: Digitized experimental data of boroxol ring fraction[3] and viscosity[1] against density for $B_2O_3$. Data is curated from $B_2O_3$ at various temperatures. The figure captures the difficulty in achieving large boroxol fractions in equilibrium MD simulations. Boroxol ring fractions greater than 30% grow in the supercooled liquid at forbiddingly large viscosity values, i.e., large structural relaxation times. Sampling of configurations at such large viscosities through equilibrium MD simulations is challenging.

## S2 Summary of Simulations Literature on Boroxol Yield in $B_2O_3$ Glasses

Table S1 summarizes efforts in the literature on simulations of $B_2O_3$ glass and, in particular, on their boroxol ring fractions.

Table S1: Summary of efforts in literature to model $B_2O_3$ glass using force field (FF).

| S. No. | Force field (FF) type | Boroxol fraction (%) | Remarks | References |
|---|---|---|---|---|
| 1 | 2-body interaction | 0 | absence of directional forces | [4] [5] [6] [7] [8] [9] [10] |
| 2 | 3-body interaction | 0-53 | Disagreement in structure factor | [11] [12] [13] [14] |
| 3 | 4-body interaction | 3.6 | Disagreement in structure factor | [15] |
| 4 | FF from Crystallization | 25-53 | density -10 to -36% off | [16] |
| 5 | Hybrid MD/MC | 74 | not stable under DFT equilibration | [17] |
| 6 | Polarizable | 1-12 | coordination defect | [18] |
| 7 | 3+4 body interaction | 17 | boroxol fraction decreases with increasing system size | [19] |

# S3 MLP Refinement

In our previous work on the development of an MLP for $B_2O_3$ glass at high pressure[20] using the DeePMD package,[21,22] we primarily focused on the properties of the glass at high pressures. Thus, configurations rich in boroxol rings, which are experimentally reported to prevail at ambient conditions, were not intentionally included in the training set. This could be one of the reasons why our model (ML-26/R6 with 1700 atoms) was not able to predict the experimentally reported fraction of boron atoms in boroxol rings ( 75%); instead, its prediction was around 15-20% .[20] In subsequent ML generations (ML-25 to ML-30), we added a large number of boroxol-rich configurations to the training dataset, which resulted in a marginal increase in the percentage of boroxol fraction in the melt-quenched glass, albeit significantly less than the experimental value. In the following, we describe the process of obtaining these configurations with high boroxol content.

## S3.1 High Boroxol Dataset Collection

The high boroxol frames were collected from different MD simulations (carried out under various conditions: constant-NVT, constant-NPT, and ramping of either temperature or pressure), starting from initial crystalline configurations containing 50% and 100% boroxol fractions, which were computer-generated by Ferlat et al. [23] In particular, two crystal structures (T10 with 50% boroxol and T3-b with 100% boroxol at densities 1.49 and 0.93 g/cc, respectively)[23] were collected from their Supporting Information, and the stability of those crystals was checked with MLP-26. We found that these crystals were stable up to 2000 K. Therefore, we applied pressure to the systems at a temperature of 1600 K to achieve a glass density of 1.834 g/cm$^3$. In this process, some of the boroxol rings melted, and the ensuing configurations contained boroxol fractions of approximately 45% and 90% for the T10 and T3-b crystals, respectively. 670 frames ranging in density between 1 to 2 g/cc were sampled from the above NVT and NPT trajectories. Further, in ML-30, we removed all

frames whose density was higher than 2.4 g/cc, as structures within them were presumed to be irrelevant to the study of the glass at 1.834 g/cc. Additionally, we included 153 samples from $B_2O_3$-I at a temperature of 300 K, 99 samples from $B_2O_3$-II at 300 K, and 99 samples from a glass with a density of 3.6 g/cc, heated to 2400 K.

Figure -S3 illustrates key characteristics of the frames sampled for the development of the machine-learned potential, ML-31. The fraction of boron atoms present in boroxol rings is plotted against density. The samples span a density range of 1.0 g/cc to 2.4 g/cc, covering all boroxol fractions up to 75%.

Those frames are collected through the following procedures:

1. First, a configuration with 90% boroxol was taken at 300 K with the glass density (1.8 g/cc).

2. The sample was melted by increasing the temperature from 300 K to 2000 K under constant-NVT conditions at a rate of $10^{11}$ K/s.

3. From the above trajectory, 12 different configurations were chosen at various fractions of boroxol, ranging from 90% to 35% at an interval of 5%.

4. Using them as initial configurations, 12 independent NPT simulations were run at a temperature of 300 K with their pressures ramped from 0 to 5 GPa.

5. Again, 12 more independent NPT simulations were run at 300 K with pressure ramping from 0 to -3 GPa, each run lasting for 10 ns.

6. From the above runs, a total of 1350 frames were collected and added to the training set of ML-31.

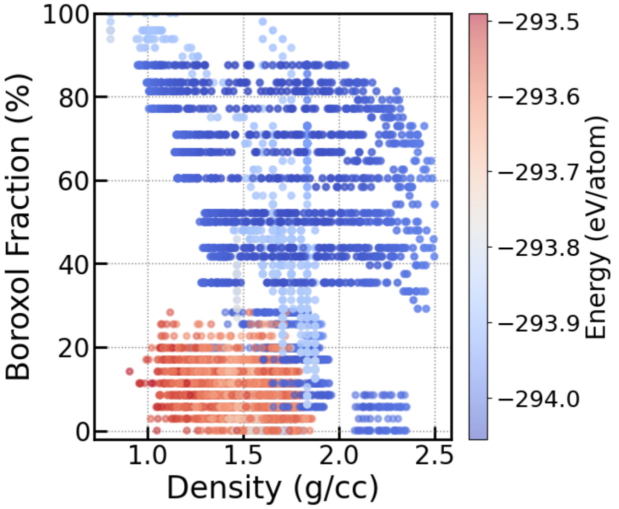


Figure S3: Scatter plot of density and boroxol fraction of 7427 frames constituting the training data set leading to ML-31 MLP. The remaining 351 frames of the training dataset, comprising 7,778 configurations, are devoid of boroxol rings and were taken from various crystalline configurations under high-pressure conditions. Specifically, this includes 153 samples from $B_2O_3$-I at a temperature of 300 K, 99 samples from $B_2O_3$-II at a temperature of 300 K, and 99 samples from a glass density of 3.6 g/cc glass heated to 2400 K. These 351 frames are not presented in this figure. The color of each data point is the total DFT energy of that configuration.

## S3.2 DeePMD MLP training

We used 8652 frames to develop the model, applying an 90:10 ratio for the training and test datasets using DeePMD package,[21,22] i.e., 7778 frames for training and 874 frames for validation. Figure S4 illustrates the parity plot for energy and force. The Root Mean Square Error (RMSE) for energy and force is 2.8 meV/atom and 211 meV/Å, respectively. Additionally, the Mean Absolute Error (MAE) for energy and force is 2.07 meV/atom and 155 meV/Å, respectively.

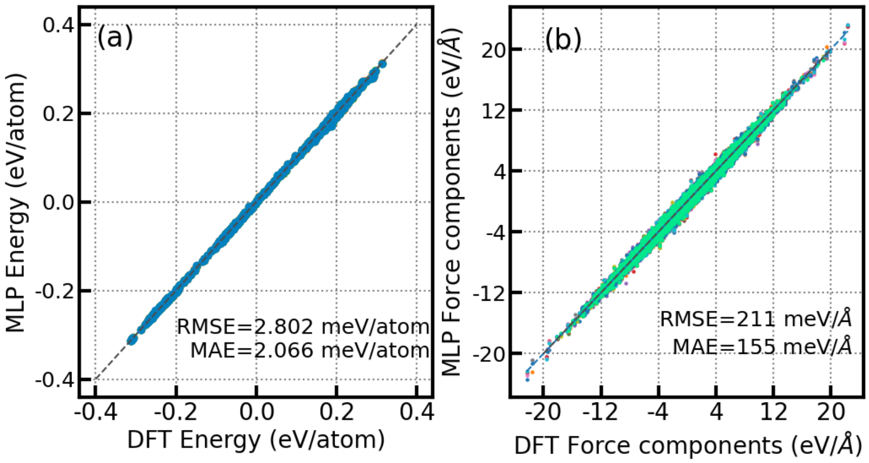


Figure S4: Parity plot of energy and force for ML-31/R6 DP MLP.

## S3.3 DeePMD Hyperparameter testing

Table S2: Accuracy of MLP was tested for different cutoff values. This indicates that the cutoff does not significantly impact the accuracy of MLPs, beyond 6 Å.

| MLP Version | neighbour list | cut-off | Train RMSE | | Validation RMSE | |
|---|---|---|---|---|---|---|
| | | | E(meV/atom) | F(meV/Å) | E(meV/atom) | F(meV/Å) |
| 30 | (100,50) | 6 | 2.73 | 224 | 2.89 | 225 |
| 31 | (100,50) | 6 | 2.66 | 214 | 2.80 | 211 |
| 31 | (100,100) | 6 | 2.67 | 212 | 2.86 | 212 |
| 31 | (100,100) | 6.5 | 2.66 | 211 | 2.83 | 208 |
| 31 | (100,100) | 7 | 2.60 | 207 | 2.76 | 205 |
| 31 | (100,100) | 7.5 | 2.59 | 205 | 2.77 | 203 |
| 31 | (100,100) | 8 | 2.59 | 204 | 2.74 | 202 |
| 31 | (100,100) | 9 | 2.62 | 204 | 2.74 | 201 |

## S3.4 MACE training

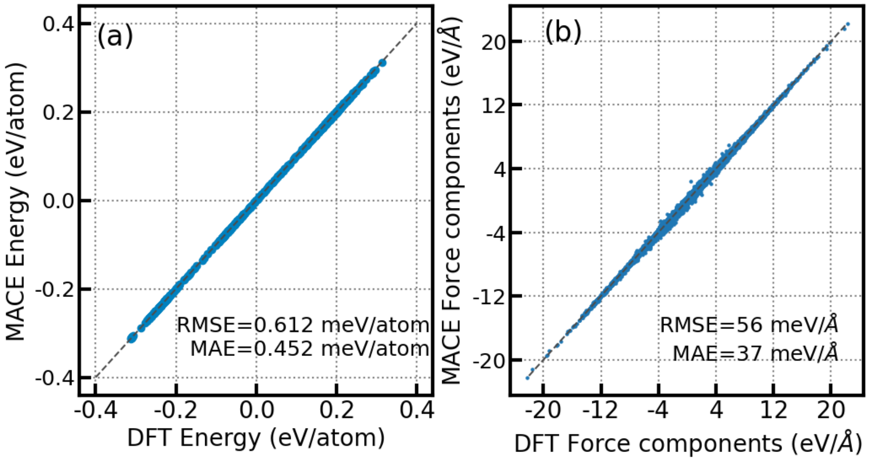


Figure S5: Parity plot of the MACE model developed on the ML-31 dataset.

## S3.5 MACE Hyperparameter testing

Table S3: Accuracy of the MACE MLP was tested for different hyperparameters.

| Precision | Channels | Interactions | Correlation | Cut-off | Validation RMSE | |
|---|---|---|---|---|---|---|
| | | | | | E(meV/atom) | F(meV/Å) |
| 64 | 64 | 2 | 3 | 6 | 0.61 | 56 |
| 64 | 64 | 2 | 3 | 4 | 1.81 | 89 |
| 64 | 64 | 2 | 3 | 3 | 5.1 | 158 |
| 32 | 64 | 2 | 3 | 4 | 1.87 | 89 |
| 32 | 64 | 1 | 3 | 4 | 3.42 | 229 |
| 32 | 64 | 2 | 2 | 4 | 2.17 | 109 |
| 32 | 32 | 2 | 3 | 4 | 1.96 | 96 |
| 32 | 16 | 2 | 3 | 4 | 2.04 | 107 |

## S4 MLP validation: Equation of State of Crystals

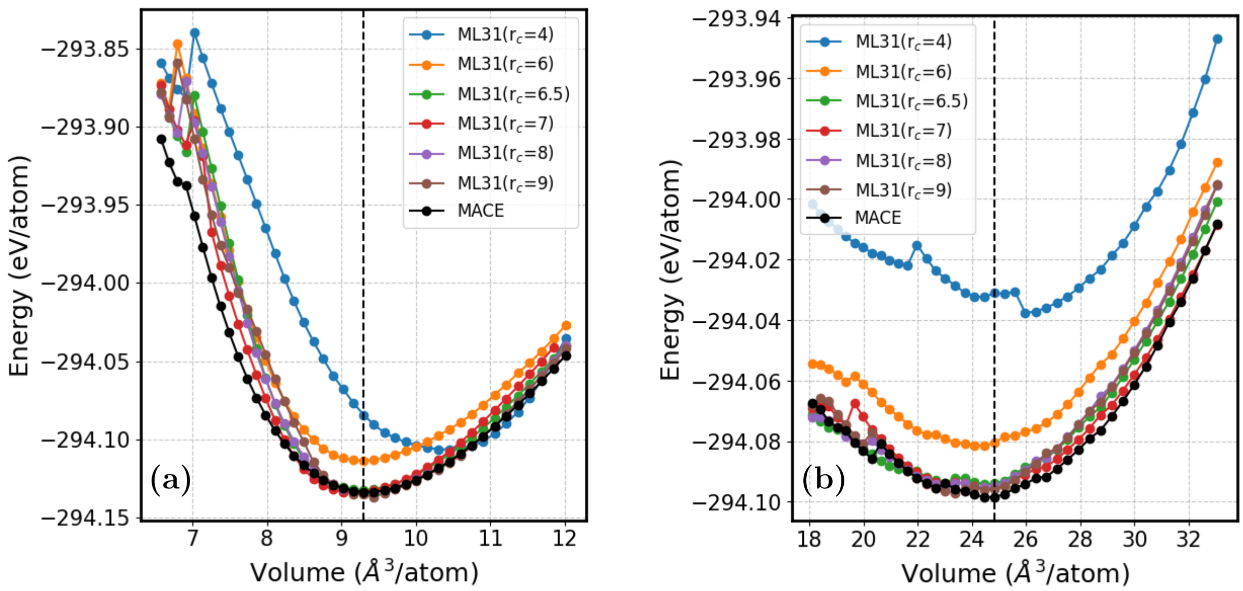


Figure S6: (a) The equation of state for the crystal $B_2O_3$-I is presented using different descriptor ranges. (b) The equation of state for the crystal $B_2O_3$-I-b is also shown with various descriptor ranges. Additionally, the results from an MACE-MLP, which was trained on the same dataset as ML-31, are included. The dashed vertical line indicates the volume at which the MACE energy reaches its minimum. It is important to note that the volume at which the ML-31/R6 energy is minimized is located to the left of this vertical line in panel (b).

Equation of state (EoS) calculations are a relatively easy test of the accuracy of the MLPs from a bulk material perspective. Figure S6 displays the equation of state (energy per atom versus volume per atom) for $B_2O_3$-I and the in-silico generated crystal, $B_2O_3$-I-b.[23] The latter was introduced by Ferlat et al[23] and was generated from $B_2O_3$-I, by replacing all its $BO_3$ units with boroxol rings, with appropriate scaling of the unit cell volume. The EoS was computed by optimizing the crystal structure and then isotropically rescaling the lengths of the supercell by up to ±10%. After obtaining the rescaled supercell and coordinates, energy minimization was performed again using the corresponding MLPs. This process allows for the determination of the lowest energy configuration at each volume. The volume corresponding to the minimum energy for the MLP with 6 Å descriptor cut-off is different from those with higher cut-offs. Thus, while the energies may be similar to those from the higher cut-off

MLPs, the volume per atom differs, suggesting that the 6 Å cut-off for the descriptor is not sufficient.

In Figure S7, we display the minimum energy and the volume at the energy minimum for all the $B_2O_3$ crystals, including several in-silico ones, using MLPs with different descriptor ranges. These were obtained by performing similar EoS calculations as shown in Figure S6 for the crystals. In Figure-S7a, the minimum energies of the EoS are plotted against the distance cut-off of the machine learning potential (MLP) descriptor. By plotting these values against the descriptor cut-off for different crystals, it is evident that configurations with a cut-off of 6 Å or lower exhibit higher energies. To set a reference point, the energy of the 9 Å MLP was subtracted from all other MLP energies for the same crystal, effectively calibrating the reference energy to zero. The shaded region shows the ±5 meV/atom deviation from the 9 Å MLP energy values. Panel (b) displays the same as (a), but for the volume per atom at the energy minimum, as a function of descriptor cut-off. Here, to set a reference point, each volume per atom was divided by the volume per atom of MLP with a 9 Å cut-off. The shaded region shows the 2% deviation from the reference value. The MLPs with a 6 Å cut-off cannot accurately capture the correct structural environment in these crystals either, resulting in higher energies. Upon closer inspection, it can be observed that some crystals show good agreement in energy with MLPs using higher cut-off values, even with the 6 Å cut-off. However, this is not true across the board, as illustrated in Figure S6. Thus, a descriptor range of at least 9 Å is required for the embedding network of DPMD for an accurate description of the atomic configuration and its mapping to the energy.

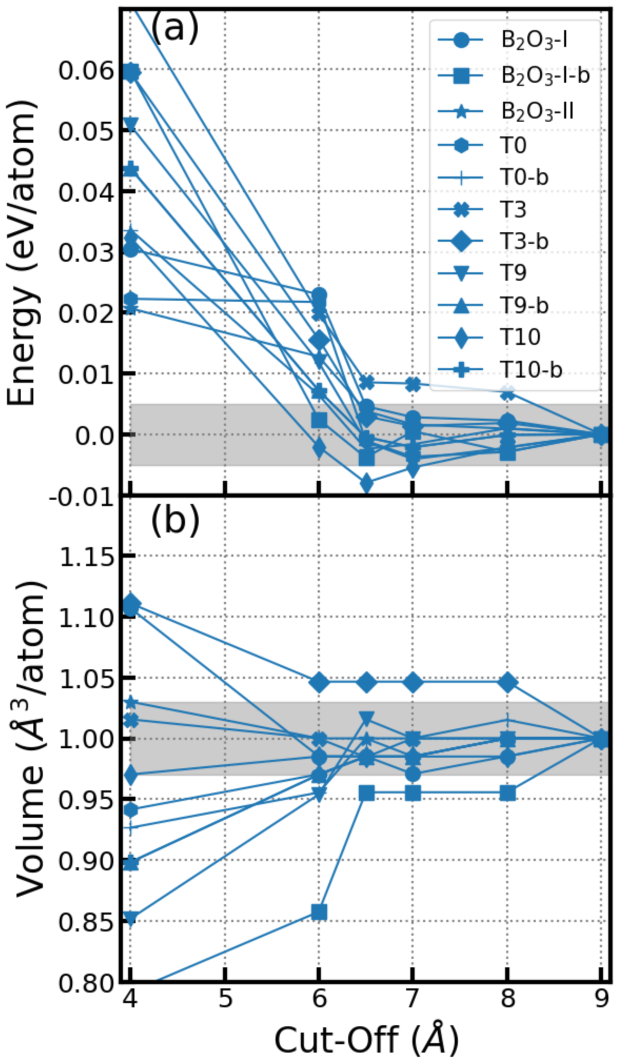


Figure S7: Equations of state (EoS) are smooth convex (U-shaped) curves which are plotted as E (eV/atom) versus V (Å$^3$/atom) of the unit cell. The minima $(E_o, V_o)$ of these curves are of interest to us. Each MLP gives a distinct EoS, which can be characterised by $E_o, V_o$ values and those are plotted in panels (a) and (b), respectively. Illustrative EoS of two $B_2O_3$ crystals are displayed in Figure S6.

## S4.1 Pressure versus MLP descriptor range cut-off

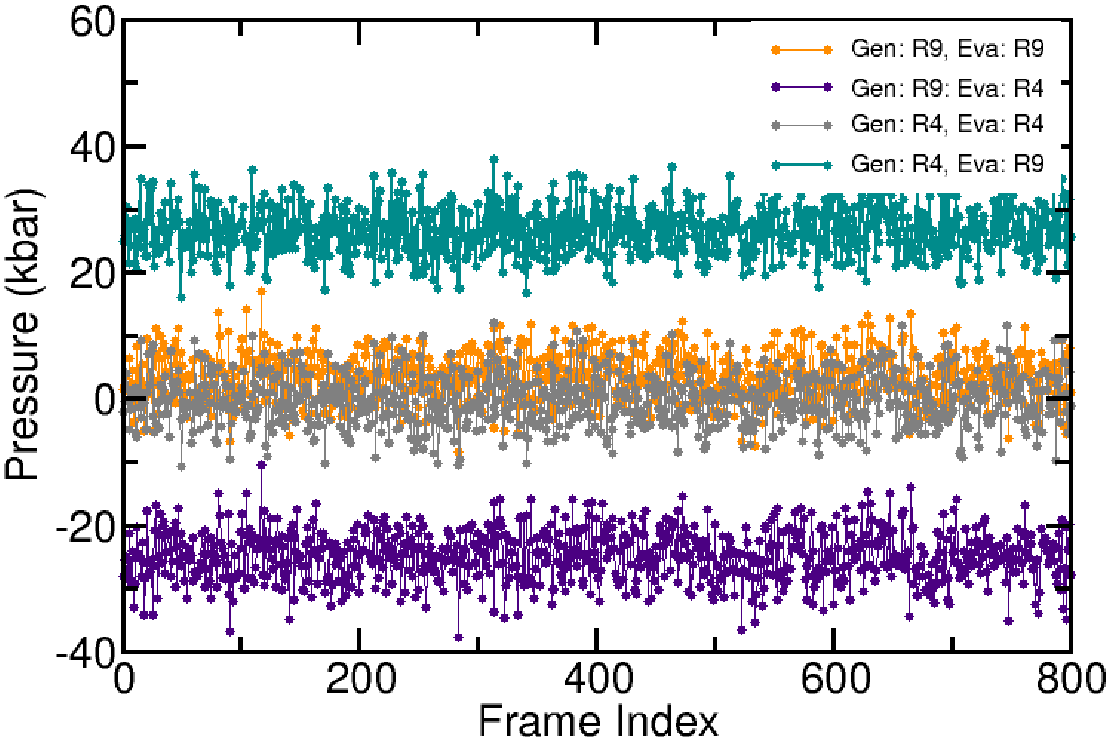


Figure S8: In Figure 2b of the main manuscript, results of pressure of the $B_2O_3$ melt at 2400 K & 1.49 g/cc, modeled with DP models of different descriptor ranges were provided. Here, we display the pressure of the trajectory generated with the ML-31/R4 model evaluated by the ML-31/R4 and ML-31/R9 models, denoted in legend as "Gen: R4, Eva: R9" and "Gen: R4, Eva: R9" respectively. Likewise, the pressure of the trajectory generated with ML-31/R9 model evaluated by ML-31/R9 and ML-31/R4 model, denoted in legend as "Gen: R9, Eva: R9" and "Gen: R9, Eva: R4" respectively.

# S5 Structural Analysis

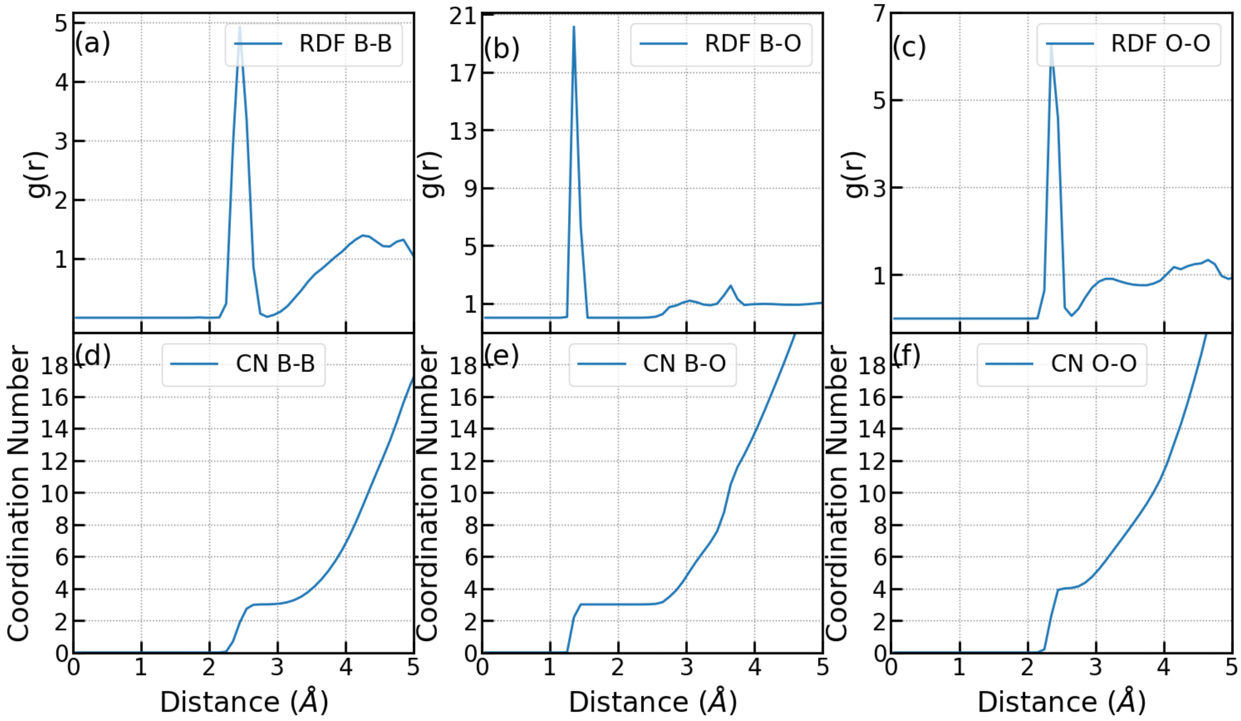


Figure S9: Radial distribution function and running coordination number of $B_2O_3$ glass at 300 K using ML-31/9A with a system size of 1700 atoms, obtained at a quenching rate of $1.6 \times 10^{11}$ K/s. The data is averaged over four independent runs.

As ML-26 was trained for high-pressure glassy $B_2O_3$, it was able to capture the change in not only the boron-oxygen coordination number with increasing density, but also describe the local geometry rather well. ML-31 also contained a good number of frames with four-coordinated boron atoms. Thus, it too possesses the capability to capture coordination changes of boron. At 1.834 g/cc, only three-coordinated boron atoms exist (Figure -S10), while at a higher density (say, at 2.854 g/cc), both four- and three-coordinated boron atoms are present.At 1.834 g/cc, the mean B-O bond length in the glass is the same as the average B-O bond length in the $B_2O_3$-I crystal.[24,25]

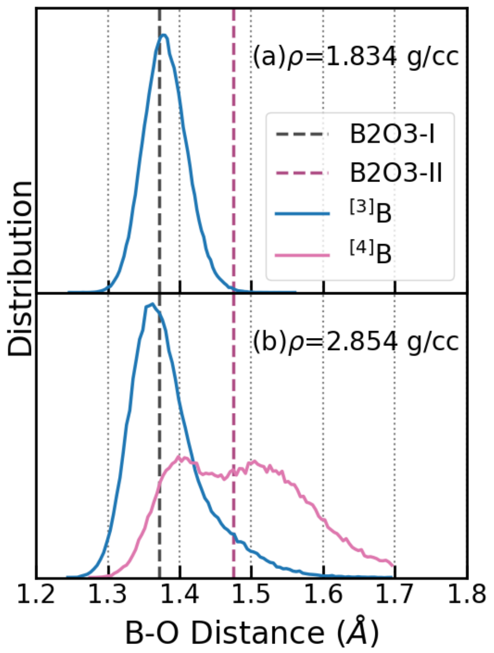


Figure S10: The coordination number transformation in $B_2O_3$glass captured by ML-31, at 300 K, obtained after quenching from 2400 K at a quench rate of $10^{11}$ K/s. The distributions show the B-O bond length distributions for 3-coordinated ($^{[3]}$B) and 4-coordinated ($^{[4]}$B) boron atoms in glassy $B_2O_3$. The dashed lines show the average B-O bond distance in two different crystalline forms, $B_2O_3$-I and $B_2O_3$-II. ML-26 also displays a similar behavior.

However, at 2.854 g/cc, the B-O bond length distribution in glassy $B_2O_3$ displays two peaks. The one at 1.52 Å is contributed by four-coordinated, tetrahedral species; the distance tallies with the B-O bond length found in $B_2O_3$-II crystal, which contains only tetrahedrally connected boron atoms. The one at 1.4 Å is contributed by three-coordinated, trigonal boron atoms. The changes in coordination number of boron that are seen at high pressures of $B_2O_3$ glass are observed at ambient conditions in sodium borosilicate glass.[26] This underscores the need for a precise modeling of these transformations in the glass structure.

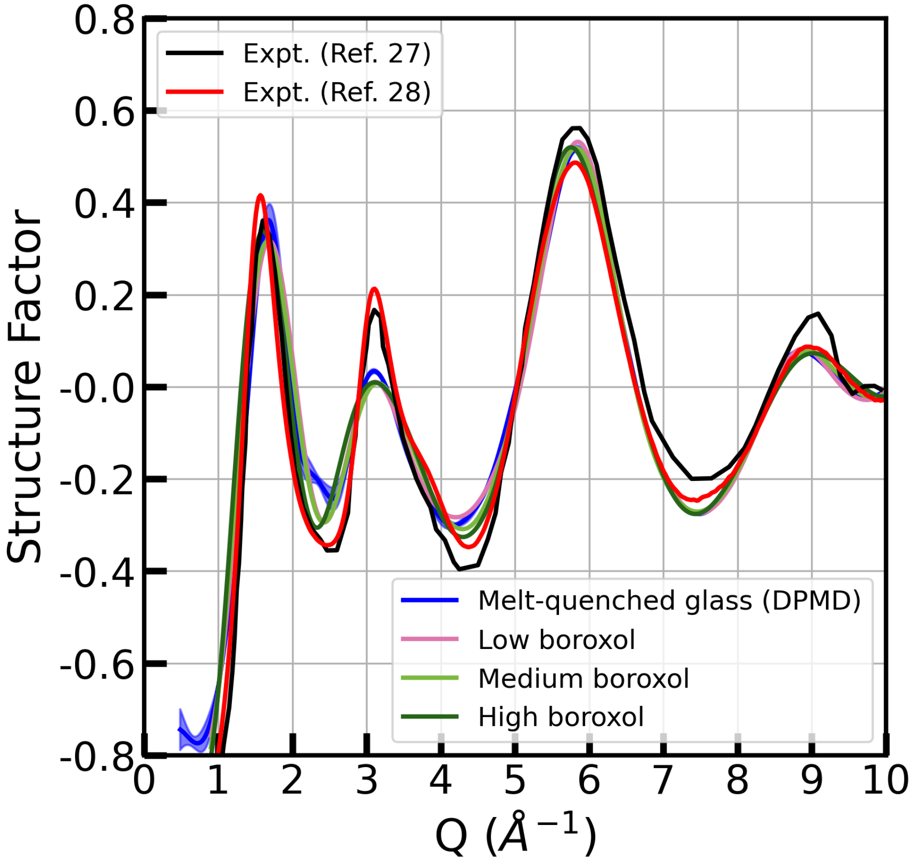


Figure S11: X-ray structure factor was calculated for the amorphous structures at 1.834 g/cc obtained through the procedure described in Figure S20. High boroxol: 60% to 100%, Medium boroxol: 40% to 60%, Low boroxol: 0% to 40%. The experimental data is reproduced from Ref.[27,28] Shown also is the same quantity for the melt-quenched glass modeled with ML-31/R9 containing 25% boroxol ring fraction. Our analyses suggest that the minor deviation in the structure factor of the melt-quenched glass in the current simulation from the experimental data around 2.3Å$^{-1}$ likely arises from a relatively insufficient number of boroxol rings in the simulated sample.

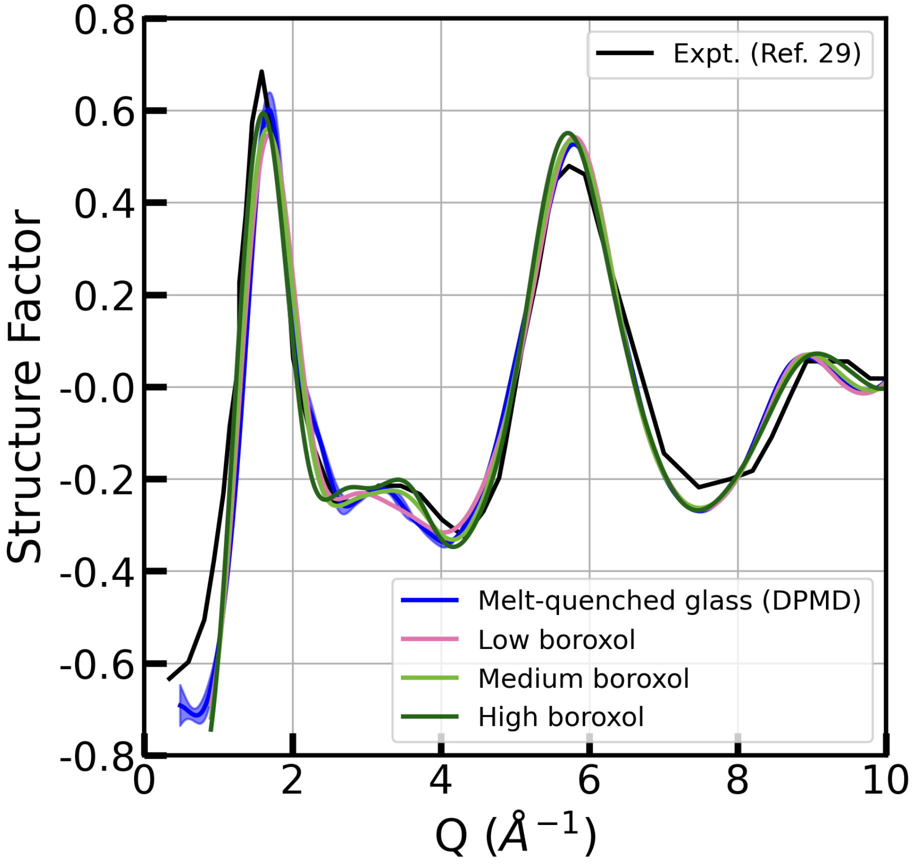


Figure S12: Neutron structure factor was calculated for the structures obtained from the melting of 100% boroxol $B_2O_3$-T3-b crystal using the procedure depicted in S20. High boroxol: 60% to 100%, Medium boroxol: 40% to 60%, Low boroxol: 0% to 40%.The experimental data were collected from literature .[29] Shown also is the same quantity for the melt-quenched glass modeled with ML-31/R9 containing 25% boroxol ring fraction. Our analyses suggest that the minor deviation in the structure factor of the melt-quenched glass in the current simulation from the experimental data around 2.3Å$^{-1}$ likely arises from a relatively insufficient number of boroxol rings in the simulated sample.

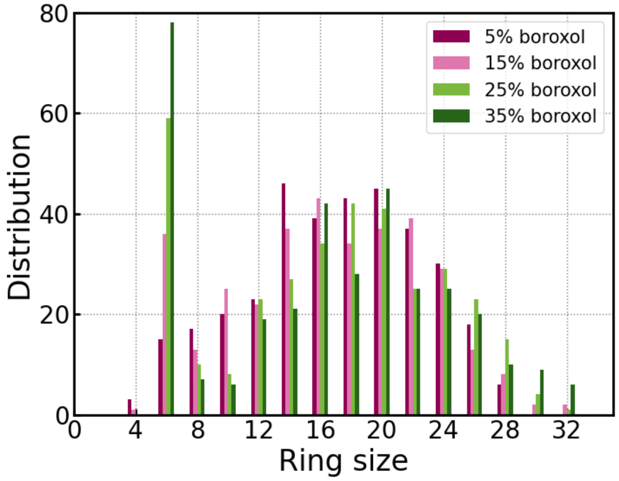


Figure S13: Distribution of ring sizes for $B_2O_3$ glasses of 1700 atoms, obtained by the melt-quenched method using ML-31/R9 MLP. With increasing boroxol fraction in the glass, rings proximal in size to boroxol (i.e., 8 and 14-membered rings) systematically decrease, while the 30-member ring increases in proportion.

# S6 Results

## S6.1 Quenching at Constant Volume: NVT

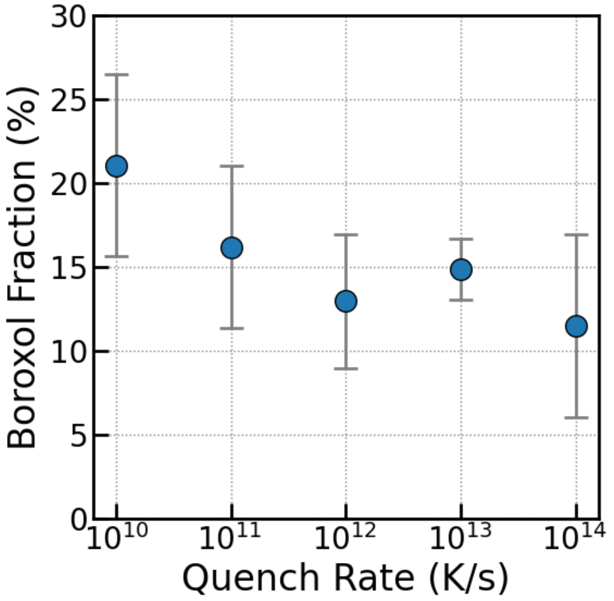


Figure S14: Fraction of boron atoms in boroxol rings in $B_2O_3$ glass at 300 K obtained by melt-quenching from 2400 K under NVT conditions at a temperature-independent density of 1.834 g/cc using the ML-26/R6 model.[20] The initial configuration was generated through random packing, followed by energy minimization using a classical force field.[30] The system was then equilibrated for 5 ns at 2400 K, consistent with our previous high-pressure melt quenching procedures. Completing a single trajectory with a quenching rate of $1 \times 10^{10}$ K/s took 20 days on a Tesla V100-SXM2-16GB using LAMMPS[31] patched with DeePMD. The reported boroxol fraction at 300 K is based on four independent runs, along with their respective standard deviations.

We attempted various methods and procedures using ML-26 to understand the dependence of boroxol fraction on them, by quenching the melt containing 1700 atoms, from high temperatures to 300 K. The following quenching rates were employed: $1{\times}10^{10}$ K/s, $1{\times}10^{11}$ K/s, $1{\times}10^{12}$ K/s, $1{\times}10^{13}$ K/s and $1{\times}10^{14}$ K/s within a NVT ensemble starting from 2400 K to 300 K. As the MLP had a committee size of four, four independent runs were performed simultaneously, each of which yielded a different fraction of boroxol rings. The maximum value of boroxol fraction obtained by this procedure was 28%. Figure S14 shows the boroxol fraction with different quenching rates.

The boroxol fraction in the training set of ML-26 was 28%. Thus, we felt that the lack of a sufficient number of rich boroxol frames could probably have made the MLP inadequate.

## S6.2 Results: Variable Quench Rates

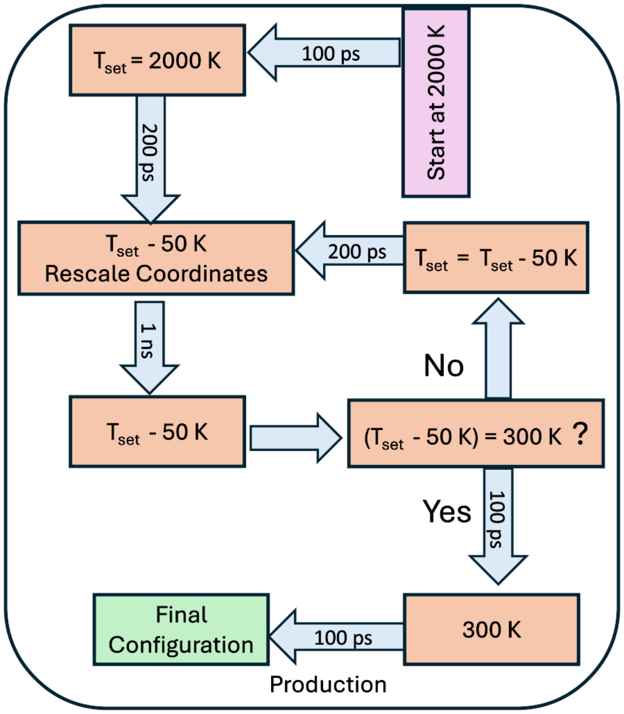


Figure S15: Constant-NVT, step-wise quenching procedure illustrated here utilises the density versus temperature curve reported in experiment (see Figure S1 in SI).[1] This procedure is termed as NVT-$\boldsymbol{\rho}_{\mathrm{EXP}}$ in the current manuscript. The initial random configuration was generated using PACKMOL ,[32] followed by energy minimization employing a classical force field ,[30] starting at 2000 K. Once the system attained 300 K, a production run was conducted, following a 100 ps equilibration. The specific time durations mentioned in this figure makes for an effective quench rate of $4 \times 10^{10}$ K/s.

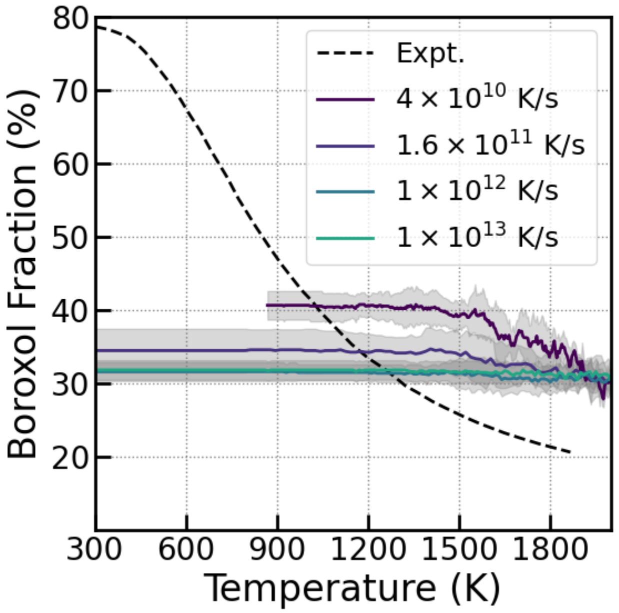


Figure S16: The boroxol fraction as a function of temperature was analyzed in DPMD simulations using ML-31/R6 for four different quenching rates. Solid lines represent the average results from four independent runs, while the shaded grey regions indicate the standard deviation across these runs. The dashed black line corresponds to the experimental boroxol fraction estimated by Walrafen et al.[33] In their study, the Raman intensity at 800 $cm^{-1}$ was used as an indicator of the boroxol percentage, modeled by the equation: $\ln\left(\frac{f(T)}{A-f(T)}\right) = \frac{B}{T} + C$, In this equation, the constants A, B, and C have the following values: A = 0.7882, B = 2490.5 K, and C = -2.3734.

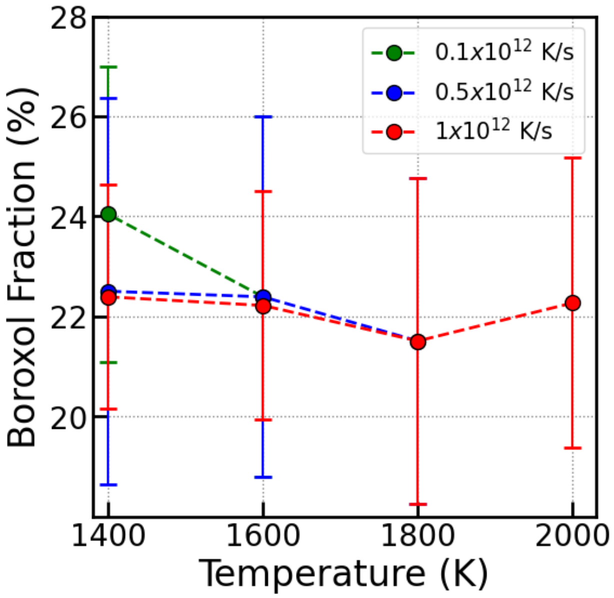


Figure S17: Boroxol fraction with variable quench rate. Three different quench protocols were attempted. In one, a constant quench rate of $1\times10^{12}$ K/s was used from 2000 K to 1400 K. In a second simulation, a quench rate of $1\times10^{12}$ K/s was used from 2000 K to 1800 K which was reduced to $0.5\times10^{12}$ K/s from 1800 K to 1400 K. A third simulation was performed with a quench rate of $1\times10^{12}$ K/s from 2000 K to 1800 K and $0.5\times10^{12}$ K/s from 1800 K to 1600 K and $0.1\times10^{12}$ K/s from 1600 K to 1400 K. Each of these simulations contained four independent runs. These simulations were performed under NVT-$\boldsymbol{\rho}_{\mathrm{EXP}}$ conditions using the ML-31/R9 MLP.

## S6.3 Vibrational Spectra

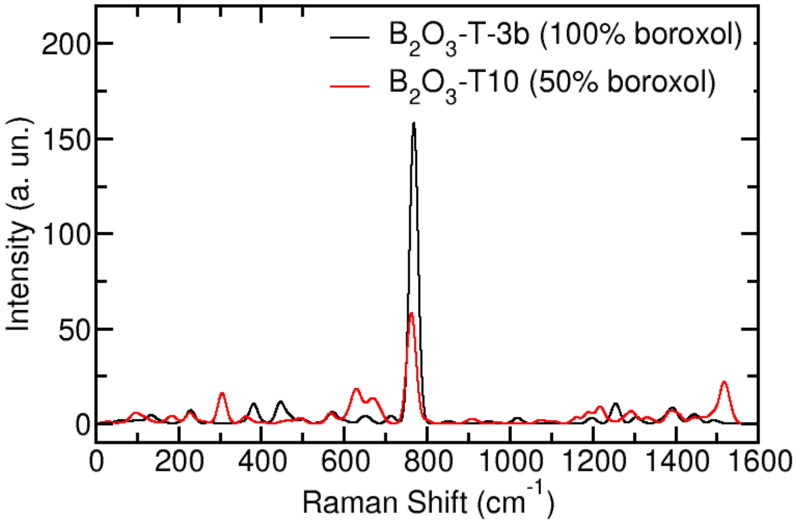


Figure S18: Raman spectra of two in-silico generated crystals proposed by Ferlat and coworkers,[23] calculated using the DFPT method implemented in Quantum Espresso[34,35] for a system size of 45 atoms of $B_2O_3$T-3b and 30 atoms of $B_2O_3$T10 at LDA level of theory. The boroxol breathing mode displays a strong peak at 765 $cm^{-1}$.

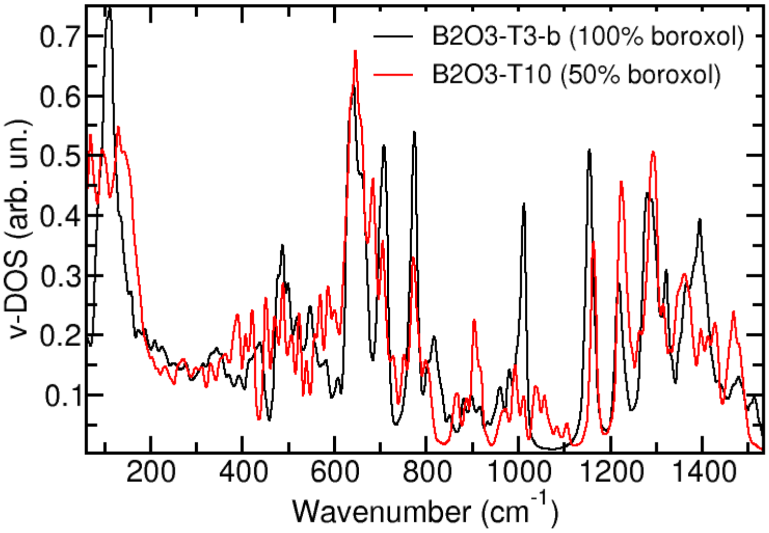


Figure S19: Vibrational density of states (VDOS) of the two in-silico generated crystals obtained from a DPMD trajectory using the ML-31/R9 model. The boroxol breathing mode displays a strong peak at 774 $cm^{-1}$.

## S6.4 Generation of amorphous configurations over a wide range of boroxol fractions

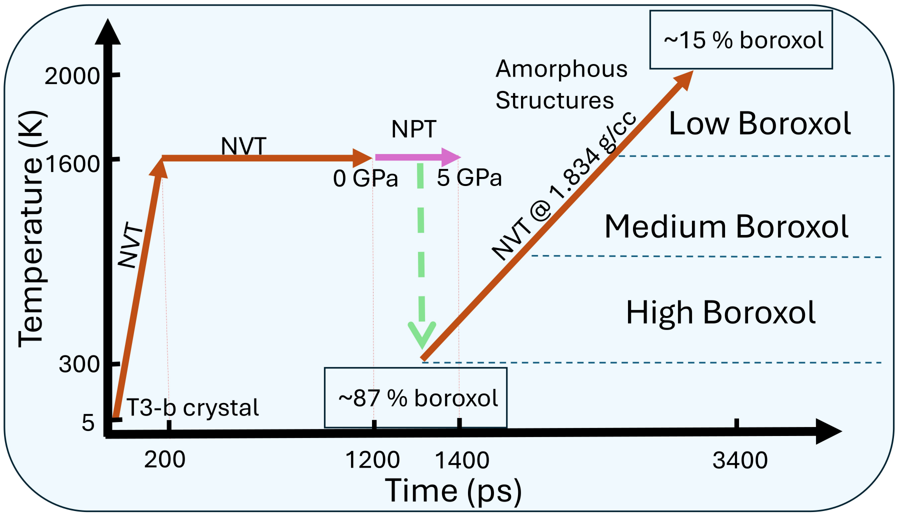


Figure S20: A total of 300 amorphous configurations with varying boroxol concentrations were collected by following the procedure illustrated here. The in-silico crystal T3-b, which contains 100% boroxol, was obtained from the literature .[23] Using the DeePMD potential, the crystal was simulated with a temperature ramp from 5 K to 1600 K over a period of 200 ps, under constant-NVT conditions. The system was then equilibrated for 1 ns at 1600 K. Following this, an NPT simulation was conducted, applying a pressure ramp of 5 GPa over 200 ps to generate frames with high boroxol content at a glass density of 1.834 g/cc. From the frame with a density of 1.834 g/cc and a boroxol fraction of approximately 87%, an NVT simulation was performed, increasing the temperature from 300 K to 2000 K to melt the boroxol rings and obtain frames with varying boroxol content. In total, 300 frames were collected, with 100 frames coming from each of three different regions: low boroxol, medium boroxol, and high boroxol.(Note: This figure is not to scale)

## S6.5 Boroxol Formation Visualization

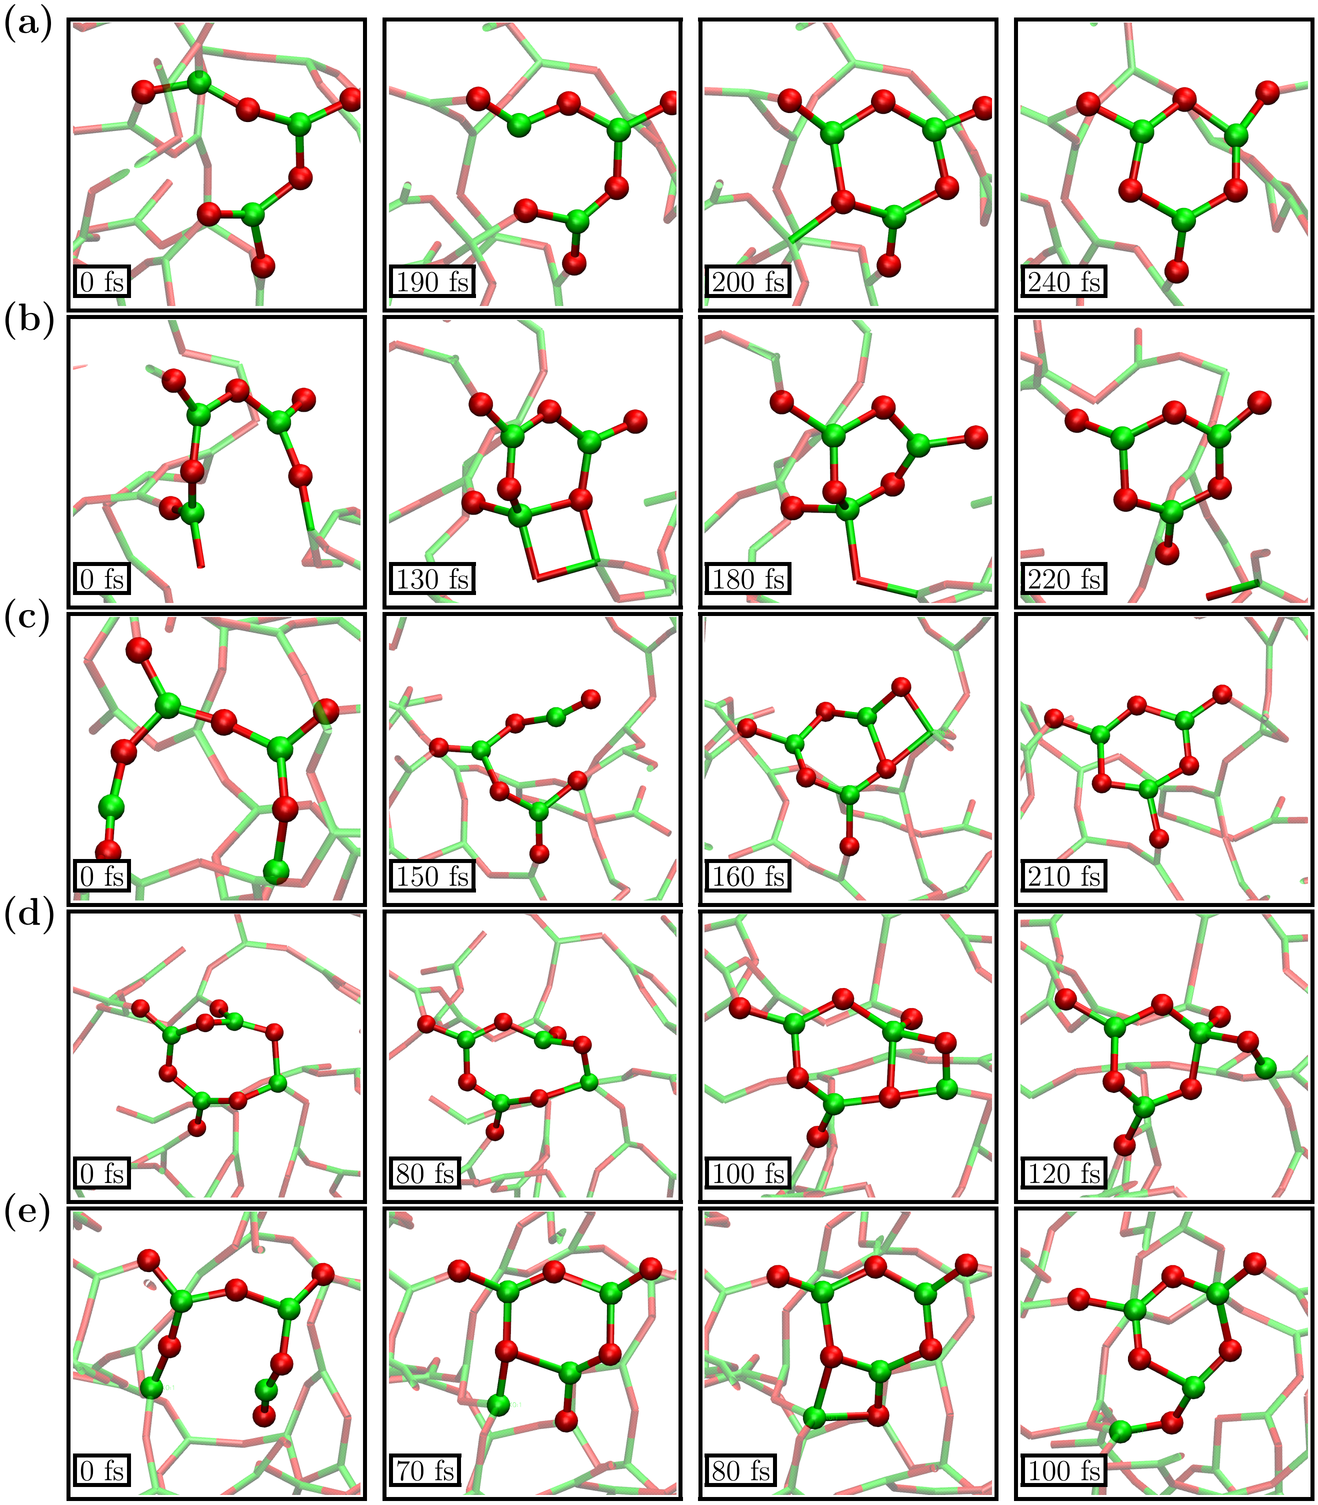
(a)
0 fs
190 fs
200 fs
240 fs
(b)
0 fs
130 fs
180 fs
220 fs
(c)
0 fs
150 fs
160 fs
210 fs
(d)
0 fs
80 fs
100 fs
120 fs
(e)
0 fs
70 fs
80 fs
100 fs

(continued)

(f)

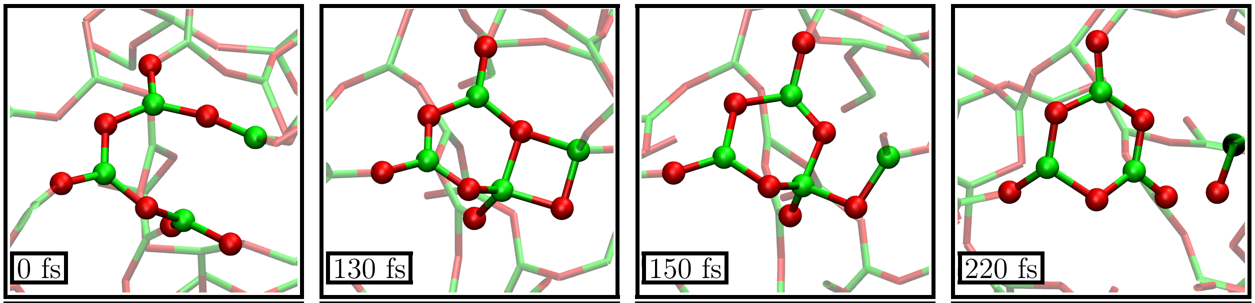


(g)

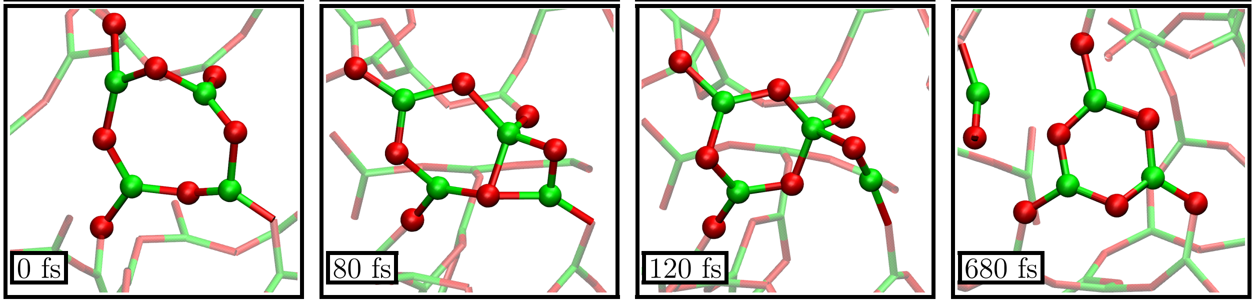


Figure S20: Additional representative boroxol formation events observed during the DPMD trajectory at 2000 K containing 1700 atoms, generated using ML-31/R9 MLP.

## S6.6 Boroxol Melting

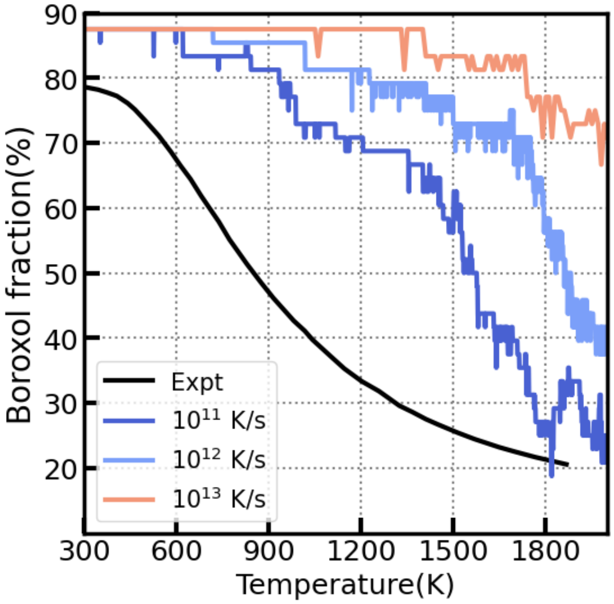


Figure S21: Evolution of boroxol ring fraction in $B_2O_3$ glass with increasing temperature at different heating rates. Experimental data is from Ref.[3]

To better understand the growth of boroxol rings with decreasing temperature and their dependence on quench rate, early on in our project, we carried out a DPMD simulation (with

the ML-28/R6 model containing 1700 atoms). In this effort, we considered an amorphous configuration of $B_2O_3$ containing 80% boroxol fraction at a density of 1.84 g/cc. The starting temperature was 300 K. The temperature of the system was increased to 2000 K at different heating rates, maintaining the same density, and the melting of boroxol rings was observed. The melting of boroxol rings is highly dependent on the heating rates (see S21), as much as their formation was dependent on the quenching rate. At the fastest melting rate, $10^{13}$ K/s, studied here, the boroxol begins to melt above 1300 K. In contrast, melting of boroxols began at approximately 500 K, at a heating rate of $10^{11}$ K/s. Shown in the same figure is the evolution of the boroxol ring fraction reported in the experiment.[3] It is thus clear that a similar dependence of boroxol ring fraction in the simulations would require orders of magnitude slower heating rates (likewise orders of magnitude slower cooling rates).

## S6.7 Negative Pressure

Ferlat[36] showed that by decreasing pressure and applying negative pressure to the melt at 2000 K, the dynamics of the glassy system become faster, allowing higher boroxol concentrations to form.

Likewise, we applied negative pressure to the system, with values ranging from 0 to -1.1 GPa, at 2000 K, and continued the simulations for 1 ns. The boroxol ring fraction began to increase at 2000 K, reaching values between 25% and 30%. The density of the system decreases, the fraction of boroxol increases, and this phenomenon could be attributed to the available space allowing for rearrangement within a limited time, enabling the system to achieve lower energy configurations, specifically boroxol network structures. Notably, the crystal predicted by Ferlat,[23] consisting of 100% boroxol, contains significant porosity with a very low density of approximately 1.1 g/cc.

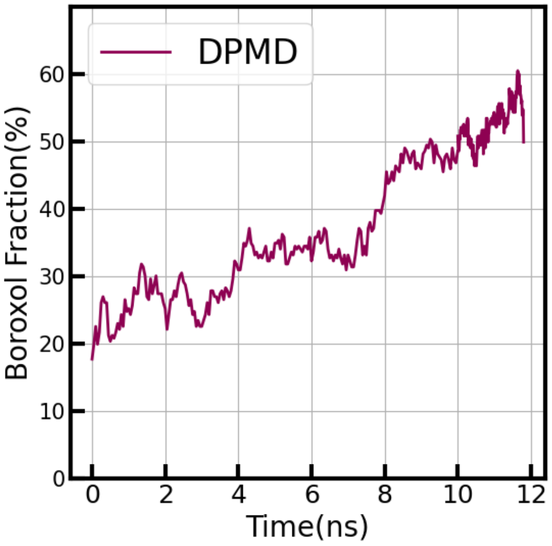


Figure S22: Boroxol fraction of the trajectory starting from 0 GPa and reaching -0.5 GPa at 2000 K using ML-31/R6 for 10 ns. Subsequently, the system was simulated for an additional 2 ns under constant-NVT at 2000 K.

By using DeePMD at 2000 K, a 10 ns MD simulation was conducted with pressure quenching from 1 bar to -1 GPa. The results showed that the boroxol fraction increased from 20% to 50% during the quenching process. After performing an equilibration run at

the final thermodynamic points, the boroxol fraction rose to 60% within 2 ns. The mean squared displacement (MSD) at 2000 K over the 10 ns duration was 2.5 $nm^2$/10 ns.

This observation demonstrates that with an increase in volume, the network relaxes into its most stable configurations. The boroxol fraction with time in this run is shown in Figure-S22.

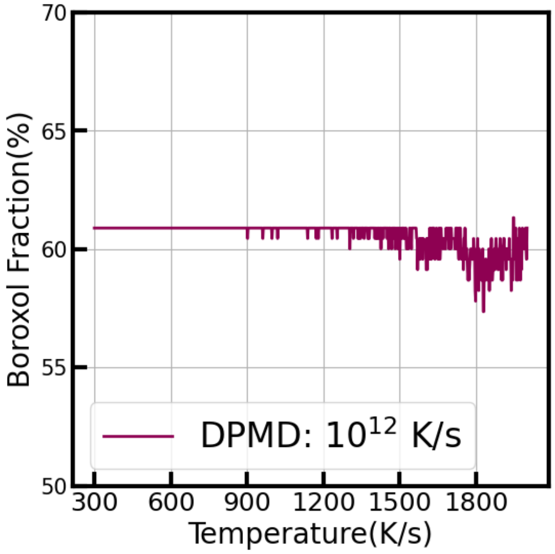


Figure S23: Boroxol fraction in a simulation initiated from an amorphous high-temperature (2000 K) melt, rich in boroxol rings, modeled using ML-31/R6. It was quenched to 300 K at a rate of $10^{13}$ K/s, and subsequently, the glass density was attained by applying pressure. The figure displays the boroxol fraction during the quenching stage.

To achieve a high boroxol fraction at ambient temperature, pressure, and density, we implemented a temperature ramp followed by pressure ramping to attain the correct density. Starting from frames containing 60% boroxol, we performed temperature quenching from 2000 K to 300 K at a quenching rate of $10^{13}$ K/s, and the boroxol content remained constant at 60% as shown in Figure-S23. To obtain the glass density at room temperature, we applied a pressure of 1 GPa to the system. The pressure ramping was conducted from 0 to 1 GPa over 1 ns, which resulted in a density of 1.85 g/cc at 300 K, which is shown in Figure-S24. Throughout this process, the boroxol content did not change significantly, yielding a final value of 57%. This exercise indicates that a high boroxol fraction can be achieved by following different quenching pathways.

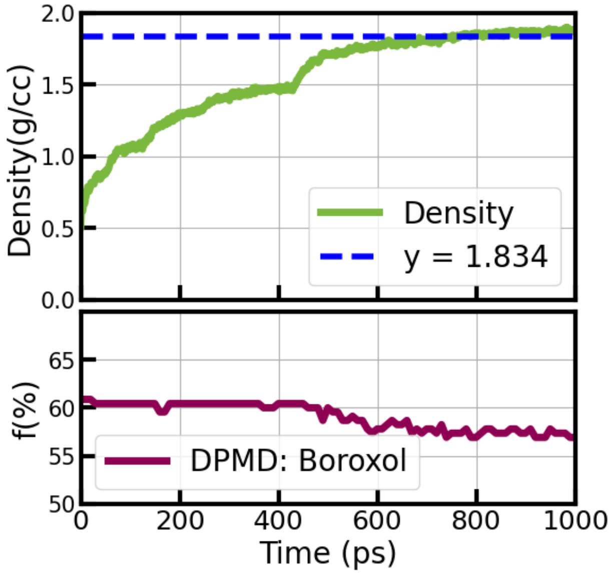


Figure S24: Same procedure as in Figure S23, but for the second stage, i.e., the application of pressure at 300 K to attain the desired density of 1.834 g/cc. The evolution of density and boroxol ring fraction, f, are shown in the two panels.

# References


(1) Napolitano, A.; Macedo, P. B.; Hawkins, E. G. Viscosity and Density of Boron Trioxide. *Journal of the American Ceramic Society* **1965**, *48*, 613–616.

(2) Macedo, P. B.; Napolitano, A. Inadequacies of Viscosity Theories for B2O3. *The Journal of Chemical Physics* **1968**, *49*, 1887–1895.

(3) Walrafen, G. E.; Samanta, S. R.; Krishnan, P. N. Raman investigation of vitreous and molten boric oxide. *The Journal of Chemical Physics* **1980**, *72*, 113–120.

(4) Soules, T. F. A molecular dynamic calculation of the structure of sodium silicate glasses. *The Journal of Chemical Physics* **1979**, *71*, 4570–4578.

(5) Soules, T. F. A molecular dynamic calculation of the structure of B2O3 glass. *The Journal of Chemical Physics* **1980**, *73*, 4032–4036.

(6) SOULES, T. F.; VARSHNEYA, A. K. Molecular Dynamic Calculations of A Sodium Borosilicate Glass Structure. *Journal of the American Ceramic Society* **1981**, *64*, 145–150.

(7) Amini, M.; Mitra, S. K.; Hockney, R. W. Molecular dynamics study of boron trioxide glass. *Journal of Physics C: Solid State Physics* **1981**, *14*, 3689.

(8) Xu, Q.; Kawamura, K.; Yokokawa, T. Molecular dynamics calculations for boron oxide and sodium borate glasses. *Journal of Non-Crystalline Solids* **1988**, *104*, 261–272.

(9) Soppe, W.; den Hartog, H. A molecular dynamics study of (B2O3)1-x-y(Li2O)x(Li2Cl2)y and (B2O3)1-x-y(Li2O)x(Cs2O)y. *Journal of Non-Crystalline Solids* **1989**, *108*, 260–268.

(10) Soppe, W.; van der Marel, C.; van Gunsteren, W.; den Hartog, H. New insights into the structure of B2O3 glass. *Journal of Non-Crystalline Solids* **1988**, *103*, 201–209.

(11) INOUE, H.; AOKI, N.; YASUI, I. Molecular Dynamics Simulation of the Structure of Borate Glasses. *Journal of the American Ceramic Society* **1987**, *70*, 622–627.

(12) Verhoef, A.; Den Hartog, H. Molecular Dynamics simulations of borate glasses. *Radiation Effects and Defects in Solids* **1991**, *119*, 493–498.

(13) Verhoef, A.; den Hartog, H. A molecular dynamics study of B2O3 glass using different interaction potentials. *Journal of Non-Crystalline Solids* **1992**, *146*, 267–278.

(14) Verhoef, A.; den Hartog, H. Isotope substitution in B2O3 glass: a molecular dynamics study. *Journal of Non-Crystalline Solids* **1994**, *180*, 102–105.

(15) Fernández-Perea, R.; Bermejo, F. J.; Enciso, E. Molecular dynamics on a realistic model for a strong glass. *Phys. Rev. B* **1996**, *53*, 6215–6224.

(16) Takada, A.; Catlow, C. R. A.; Price, G. D. Computer modelling of B2O3. II. Molecular dynamics simulations of vitreous structures. *Journal of Physics: Condensed Matter* **1995**, *7*, 8693.

(17) Takada, A. Modelling of B2O3 glass structure by coupled MD/MC simulation. *Physics and Chemistry of Glasses - European Journal of Glass Science andTechnology Part B* **2006**, *47*, 493–496.

(18) Teter, M. P. In *Borate Glasses, Crystals and Melts*; Wright, A. C., Feller, S. A., Hannon, A. C., Eds.; Society of Glass Technology: Sheffield, UK, 1997; p 407.

(19) Kashchieva, E.; Shivachev, B.; Dimitriev, Y. Molecular dynamics studies of vitreous boron oxide. *Journal of Non-Crystalline Solids* **2005**, *351*, 1158–1161, Proceedings of the International Conference on Non-Crystalline Materials (CONCIM).

(20) Meher, D.; Avula, N. V. S.; Balasubramanian, S. Slowly quenched, high pressure glassy $B_2O_3$ at DFT accuracy. *The Journal of Chemical Physics* **2025**, *162*, 044503.

(21) Wang, H.; Zhang, L.; Han, J.; E, W. DeePMD-kit: A deep learning package for many-body potential energy representation and molecular dynamics. *Computer Physics Communications* **2018**, *228*, 178–184.

(22) Zeng, J.; Zhang, D.; Lu, D.; Mo, P.; Li, Z.; Chen, Y.; Rynik, M.; Huang, L.; Li, Z.; Shi, S.; Wang, Y.; Ye, H.; Tuo, P.; Yang, J.; Ding, Y.; Li, Y.; Tisi, D.; Zeng, Q.; Bao, H.; Xia, Y.; Huang, J.; Muraoka, K.; Wang, Y.; Chang, J.; Yuan, F.; Bore, S. L.; Cai, C.; Lin, Y.; Wang, B.; Xu, J.; Zhu, J.-X.; Luo, C.; Zhang, Y.; Goodall, R. E. A.; Liang, W.; Singh, A. K.; Yao, S.; Zhang, J.; Wentzcovitch, R.; Han, J.; Liu, J.; Jia, W.; York, D. M.; E, W.; Car, R.; Zhang, L.; Wang, H. DeePMD-kit v2: A software package for deep potential models. *The Journal of Chemical Physics* **2023**, *159*, 054801.

(23) Ferlat, G.; Seitsonen, A. P.; Lazzeri, M.; Mauri, F. Hidden polymorphs drive vitrification in $B_2O_3$. *Nature Materials* **2012**, *11*, 925–929.

(24) Gurr, G. E.; Montgomery, P. W.; Knutson, C. D.; Gorres, B. T. The crystal structure of trigonal diboron trioxide. *Acta Crystallographica Section B* **1970**, *26*, 906–915.

(25) Takada, A.; Catlow, C. R. A.; Lin, J. S.; Price, G. D.; Lee, M. H.; Milman, V.; Payne, M. C. Ab initio total-energy pseudopotential calculations for polymorphic $B_2O_3$ crystals. *Physical Review B* **1995**, *51*, 1447–1455.

(26) Kato, T.; Lodesani, F.; Urata, S. Boron coordination and three-membered ring formation in sodium borate glasses: a machine-learning molecular dynamics study. *Journal of the American Ceramic Society* **2024**, *107*, 2888–2900.

(27) Brazhkin, V. V.; Katayama, Y.; Trachenko, K.; Tsiok, O. B.; Lyapin, A. G.; Artacho, E.; Dove, M.; Ferlat, G.; Inamura, Y.; Saitoh, H. Nature of the Structural Transformations in $B_2O_3$ Glass under High Pressure. *Phys. Rev. Lett.* **2008**, *101*, 035702.

(28) Alderman, O. L. G.; Ferlat, G.; Baroni, A.; Salanne, M.; Micoulaut, M.; Benmore, C. J.; Lin, A.; Tamalonis, A.; Weber, J. K. R. Liquid B2O3 up to 1700 K: x-ray diffraction and boroxol ring dissolution. *Journal of Physics: Condensed Matter* **2015**, *27*, 455104.

(29) Zeidler, A.; Wezka, K.; Whittaker, D. A. J.; Salmon, P. S.; Baroni, A.; Klotz, S.; Fischer, H. E.; Wilding, M. C.; Bull, C. L.; Tucker, M. G.; Salanne, M.; Ferlat, G.; Micoulaut, M. Density-driven structural transformations in $B_2O_3$ glass. *Phys. Rev. B* **2014**, *90*, 024206.

(30) Wang, M.; Anoop Krishnan, N.; Wang, B.; Smedskjaer, M. M.; Mauro, J. C.; Bauchy, M. A new transferable interatomic potential for molecular dynamics simulations of borosilicate glasses. *Journal of Non-Crystalline Solids* **2018**, *498*, 294–304.

(31) Thompson, A. P.; Aktulga, H. M.; Berger, R.; Bolintineanu, D. S.; Brown, W. M.; Crozier, P. S.; in 't Veld, P. J.; Kohlmeyer, A.; Moore, S. G.; Nguyen, T. D.; Shan, R.; Stevens, M. J.; Tranchida, J.; Trott, C.; Plimpton, S. J. LAMMPS - a flexible simulation

tool for particle-based materials modeling at the atomic, meso, and continuum scales. *Computer Physics Communications* **2022**, *271*, 108171.

(32) Martínez, L.; Andrade, R.; Birgin, E. G.; Martínez, J. M. PACKMOL: A package for building initial configurations for molecular dynamics simulations. *Journal of Computational Chemistry* **2009**, *30*, 2157–2164.

(33) Walrafen, G. E.; Hokmabadi, M. S.; Krishnan, P. N.; Guha, S.; Munro, R. G. Low-frequency Raman scattering from vitreous and molten $B_2O_3$. *The Journal of Chemical Physics* **1983**, *79*, 3609–3620.

(34) Giannozzi, P.; Baroni, S.; Bonini, N.; Calandra, M.; Car, R.; Cavazzoni, C.; Ceresoli, D.; Chiarotti, G. L.; Cococcioni, M.; Dabo, I.; Dal Corso, A.; de Gironcoli, S.; Fabris, S.; Fratesi, G.; Gebauer, R.; Gerstmann, U.; Gougoussis, C.; Kokalj, A.; Lazzeri, M.; Martin-Samos, L.; Marzari, N.; Mauri, F.; Mazzarello, R.; Paolini, S.; Pasquarello, A.; Paulatto, L.; Sbraccia, C.; Scandolo, S.; Sclauzero, G.; Seitsonen, A. P.; Smogunov, A.; Umari, P.; Wentzcovitch, R. M. QUANTUM ESPRESSO: a modular and open-source software project for quantum simulations of materials. *Journal of Physics: Condensed Matter* **2009**, *21*, 395502.

(35) Giannozzi, P.; Andreussi, O.; Brumme, T.; Bunau, O.; Buongiorno Nardelli, M.; Calandra, M.; Car, R.; Cavazzoni, C.; Ceresoli, D.; Cococcioni, M.; Colonna, N.; Carnimeo, I.; Dal Corso, A.; de Gironcoli, S.; Delugas, P.; DiStasio, R. A.; Ferretti, A.; Floris, A.; Fratesi, G.; Fugallo, G.; Gebauer, R.; Gerstmann, U.; Giustino, F.; Gorni, T.; Jia, J.; Kawamura, M.; Ko, H.-Y.; Kokalj, A.; Küçükbenli, E.; Lazzeri, M.; Marsili, M.; Marzari, N.; Mauri, F.; Nguyen, N. L.; Nguyen, H.-V.; Otero-de-la Roza, A.; Paulatto, L.; Poncé, S.; Rocca, D.; Sabatini, R.; Santra, B.; Schlipf, M.; Seitsonen, A. P.; Smogunov, A.; Timrov, I.; Thonhauser, T.; Umari, P.; Vast, N.; Wu, X.; Baroni, S. Advanced capabilities for materials modelling with Quantum ESPRESSO. *Journal of Physics: Condensed Matter* **2017**, *29*, 465901.

(36) Ferlat, Guillaume, In *Rings in Network Glasses: The $B_2O_3$ Case. In: Molecular Dynamics Simulations of Disordered Materials: From Network Glasses to Phase-Change Memory Alloys*; Massobrio, Carlo and Du, Jincheng and Bernasconi, Marco and Salmon, Philip S.,, Ed.; Springer International Publishing: Cham, 2015; Chapter 14.
